# Supplementary material for: Capacity Achieving Modulation for Fixed Constellations with Average Power Constraint
Source: arXiv:1010.2382 source file (2011-06-27)
Supplement: Supplementary file 1 [file appendix.tex]

Define the joint distributions $r(i,y)=h_i(y)p_i$ and $r^*(i,y)=h_i(y)p^*_i$. We then have
\begin{align}
\kl(r\Vert r^*)&=\sum_i p_i\int_\mathbb{C} h_i(y)\log\frac{h_i(y)p_i}{h_i(y)p^*_i}\de y\nonumber\\
&=\kl(p\Vert p^*).\label{eq:kldev1}
\end{align}
Define now $v(i|y)$ and $v^*(i|y)$ such that $r(i,y)=v(i|y)q(y)$ and $r^*(i,y)=v^*(i|y)q^*(y)$, respectively. We then have
\begin{align}
\kl(r\Vert r^*)&=\int\sum_i v(i|y)q(y)\log\frac{v(i|y)q(y)}{v^*(i|y)q^*(y)}\de y\nonumber\\
&=\kl(q\Vert q^*)+\int_\mathbb{C}q(y)\kl[v(\cdot|y)\Vert v^*(\cdot|y)]\de y\nonumber\\
&\geq \kl(q\Vert q^*)\label{eq:kldev2}
\end{align}
where the last line follows from the information inequality \cite[Theorem 2.6.3]{Cover2006}, which states that the I-divergence between two distributions is always nonnegative. Putting together \eqref{eq:kldev1} and \eqref{eq:kldev2} yields
\begin{align}
\kl(q\Vert q^*)\leq \kl(p\Vert p^*).
\end{align}
